# Supplementary material for: Espresso: Robust Concept Filtering in Text-to-Image Models
Source: arXiv:2404.19227 source file (2025-02-26)
Supplement: Supplementary file 2 [file 10appendix.tex]

\section{Supplementary Material}\label{sec:appendix}

\subsection{Notations}\label{app:notations}

We summarize frequently used notations in Table~\ref{tab:notations}.

 \input{tables/tab_notations}


\subsection{Impact of Fine-tuning}\label{app:FTEspresso}

We present the impact of fine-tuning of \method by reporting the effectiveness (CLIP accuracy) and utility (normalized CLIP score) for all the concepts in Table~\ref{tab:FTImpact}.
We expect that fine-tuning improves utility on majority of the concepts (indicated with a higher normalized CLIP score) while maintaining the effectiveness (indicated with similar CLIP accuracy).
We use \colorbox{mynicered}{red} if effectiveness/utility degrades; \colorbox{myniceblue}{blue} if no significant change; \colorbox{mynicegreen}{green} if effectiveness/utility is better.

\input{tables/tab_nofinetune_effective}
\input{figures/fig_adversarial}

In Table~\ref{tab:FTImpact}, we observe that utility either remains the same or improves significantly for some concepts. Further, we observe that while the effectiveness remains the same for majority of the concepts, there is a benefit of fine-tuning to improve effectiveness for four concepts in Group-3 (i.e., \emph{Taylor Swift}, \emph{Angelina Jolie}, \emph{Brad Pitt}, \emph{Elon Musk}).


\subsection{Proof for Theorem~\ref{thm.1}}\label{app:proof}

We now present the full proof for Theorem~\ref{thm.1} below.

\input{proofs/proof}

\subsection{Retention of Adversarial Noise}\label{app:adv}




We present the images generated from \tti models on passing adversarial prompts corresponding to adversarial examples in Figure~\ref{fig:adversarial}.

\subsection{Efficiency of \crt{s}}\label{sec:efficiency}


In Table~\ref{tab:efficiency}, we report the execution time for fine-tuning or training the \crt{s} (average across ten runs). For related work, the configuration for fine-tuning/training is the same as specified by their respective paper to satisfy \ref{effective} and \ref{utility}. These times were obtained from training on a single NVIDIA A100 GPU.

\input{tables/tab_efficiency}

\method is reasonably fast to train.
For fine-tuning \crt{s} inference time is identical to using the baseline SD v1.4 because they do not add any additional components to the \tti generation process. The inference time for filtering \crt{s} is marginally higher (+0.01\%) than the baseline (of only the image generation time taken by the \tti model). % as it includes the inference time from both the \tti model and the filter.
