# Supplementary material for: Espresso: Robust Concept Filtering in Text-to-Image Models
Source: arXiv:2404.19227 source file (2025-02-26)
Supplement: Supplementary file 3 [file 0supplementary.tex]

% WACV 2025 Paper Template
% based on the WACV 2024 template, which is
% based on the CVPR 2023 template (https://media.icml.cc/Conferences/CVPR2023/cvpr2023-author_kit-v1_1-1.zip) with 2-track changes from the WACV 2023 template (https://github.com/wacv-pcs/WACV-2023-Author-Kit)
% based on the CVPR template provided by Ming-Ming Cheng (https://github.com/MCG-NKU/CVPR_Template)
% modified and extended by Stefan Roth (stefan.roth@NOSPAMtu-darmstadt.de)

\documentclass[10pt,twocolumn,letterpaper]{article}

%%%%%%%%% PAPER TYPE  - PLEASE UPDATE FOR FINAL VERSION
\usepackage[review,algorithms]{wacv}      % To produce the REVIEW version for the algorithms track
%\usepackage[review,applications]{wacv}      % To produce the REVIEW version for the applications track
%\usepackage{wacv}              % To produce the CAMERA-READY version
%\usepackage[pagenumbers]{wacv} % To force page numbers, e.g. for an arXiv version

% Include other packages here, before hyperref.
\usepackage{graphicx}
\usepackage{amsmath}
\usepackage{amssymb}
\usepackage{booktabs}
% It is strongly recommended to use hyperref, especially for the review version.
% hyperref with option pagebackref eases the reviewers' job.
% Please disable hyperref *only* if you encounter grave issues, e.g. with the
% file validation for the camera-ready version.
%
% If you comment hyperref and then uncomment it, you should delete
% ReviewTempalte.aux before re-running LaTeX.
% (Or just hit 'q' on the first LaTeX run, let it finish, and you
%  should be clear).
\usepackage[pagebackref,breaklinks,colorlinks]{hyperref}


% Support for easy cross-referencing
\usepackage[capitalize]{cleveref}
\crefname{section}{Sec.}{Secs.}
\Crefname{section}{Section}{Sections}
\Crefname{table}{Table}{Tables}
\crefname{table}{Tab.}{Tabs.}


%%%%%%%%% PAPER ID  - PLEASE UPDATE
\def\wacvPaperID{1890} % *** Enter the WACV Paper ID here
\def\confName{WACV}
\def\confYear{2025}

\input{00macros}
\includeversion{submission}
\excludeversion{arxiv}


\begin{document}

%%%%%%%%% TITLE - PLEASE UPDATE
\title{Supplementary Material: \method: Robust \underline{Co}ncept \underline{Fi}ltering in Text-to-Image Models}

\author{First Author\\
Institution1\\
Institution1 address\\
{\tt\small firstauthor@i1.org}
% For a paper whose authors are all at the same institution,
% omit the following lines up until the closing ``}''.
% Additional authors and addresses can be added with ``\and'',
% just like the second author.
% To save space, use either the email address or home page, not both
\and
Second Author\\
Institution2\\
First line of institution2 address\\
{\tt\small secondauthor@i2.org}
}
\maketitle

\input{WACV/10appendix}


%------------------------------------------------------------------------
% \section{Final copy}

% You must include your signed IEEE copyright release form when you submit your finished paper.
% We MUST have this form before your paper can be published in the proceedings.

% Please direct any questions to the production editor in charge of these proceedings at the IEEE Computer Society Press:
% \url{https://www.computer.org/about/contact}.


%%%%%%%%% REFERENCES
{\small
\bibliographystyle{ieee_fullname}
\bibliography{egbib}
}

% 

\end{document}
